# Supplementary material for: Instruction Induction: From Few Examples to Natural Language Task Descriptions
Source: arXiv:2205.10782 source file (2022-05-22)
Supplement: Supplementary file 1 [file appendix.tex]

% \appendix

% \section{Data Construction}
% \todo{Needs edit - ignore for now.}
% \paragraph{Pluralization} In each demonstration, $y_k$ is the plural form of $x_k$, which is a singular noun. 
% A suitable instruction, e.g., ``convert each word to its plural form.''
% \paragraph{Passivization} In each demonstration, $x_k$ and $y_k$ are two sentences with the same meaning, written in active and passive voice respectively. The model is required to predict a suitable instruction, e.g., ``Write the input sentence in a passive form.''
% \paragraph{Negation} In each demonstration, $y_k$ is the negation of the input sentences $x_k$. The model is required to predict a suitable instruction, e.g., ``Negate the input sentence.''
% \paragraph{Antonyms} In each demonstration, $y_k$ is the antonym of the input word $x_k$.
% \paragraph{Synonyms} In each demonstration, $y_k$ is a synonyms of the input word $x_k$.
% \paragraph{Co-hyponyms} In each demonstration, $x_k$ is a list of words, where some of the words belong to the same category (i.e., animals), and $y_k$ contains the words from $x_k$ belonging to this category. We note that the category is not explicitly specified.
% \paragraph{Rhymes} In each demonstration, $y_k$ is a rhyme of the input word $x_k$.
% \paragraph{Larger Object} In each demonstration, $x_k$ contains two words describing animals or object of different sizes, and $y_k$ is the larger of the two input words.
% \paragraph{Sum} In each demonstration, $x_k$ contains two numbers separated by space and $y_k$ is the sum of the two.
% \paragraph{Difference} In each demonstration, $x_k$ contains two numbers separated by space and $y_k$ is the difference between the two input numbers.
% \paragraph{Number to Word} In each demonstration, $x_k$ a number written using digits (e.g., 28) and $y_k$ is the same number, written in words (e.g, twenty-eight).
% \paragraph{Translation} In each demonstration, $x_k$ a word in English and $y_k$ is its translation to a given target language. We use French, Spanish and German as target languages. 
